# Supplementary material for: Quantitative comparison of magnon transport experiments in three-terminal YIG/Pt nanostructures acquired via dc and ac detection techniques
Source: arXiv:2008.01416 ancillary file (2020-08-04)
Supplement: Supplementary file 1 [file SI_Quantitative_comparison_of_magnon_transport_experiments_in_three-terminal_YIG-Pt_nanostructures_acquired_via_dc_and_ac_detection_techniques.pdf]

# Supplementary Material: Quantitative comparison of magnon transport experiments in three-terminal YIG/Pt nanostructures acquired via dc and ac detection techniques

J. Gückelhorn,[1,2,*] T. Wimmer,[1,2] S. Geprägs,[1]
H. Huebl,[1,2,3] R. Gross,[1,2,3] and M. Althammer[1,2,†]

[1] *Walther-Meißner-Institut, Bayerische Akademie der Wissenschaften, 85748 Garching, Germany*
[2] *Physik-Department, Technische Universität München, 85748 Garching, Germany*
[3] *Munich Center for Quantum Science and Technology (MCQST), Schellingstr. 4, D-80799 München, Germany*

(Dated: July 24, 2020)

* janine.gueckelhorn@wmi.badw.de
† matthias.althammer@wmi.badw.de

## I. SAMPLE LAYOUT

Our experiments were conducted using two different devices which ran through the same fabrication process. The single crystalline (100)-oriented yttrium iron garnet films were grown via pulsed laser deposition on gadolinium gallium garnet ($Gd_3Ga_5O_{12}$, GGG) substrates. A substrate temperature of 450 °C, an oxygen pressure of 25 µbar, a laser fluence at the target of 2.0 J/cm$^2$ and a laser frequency of 10 Hz were used. The strips were patterned via e-beam lithography and the Pt was deposited on the YIG thin films using dc sputtering. In a further step, Al leads and bondpads were deposited to connect the device electrically. The first device D500, presented in the main text, consists of 5 nm thick Pt strips with a edge-to-edge distance of $d = 200$ nm and a modulator width $w_1 = 500$ nm on a 11.4 nm thick YIG film. The second device D300 consists of 3.5 nm thick Pt strips deposited on a 7 nm thick YIG film. The Pt strips have a edge-to-edge separation of $d = 200$ nm and the modulator has a width of $w_1 = 300$ nm. In both cases the injector and the detector have a width of $w_2 = 500$ nm and a length of $l_2 = 50$ µm, while the modulators have a length of $l_1 = 64$ µm.

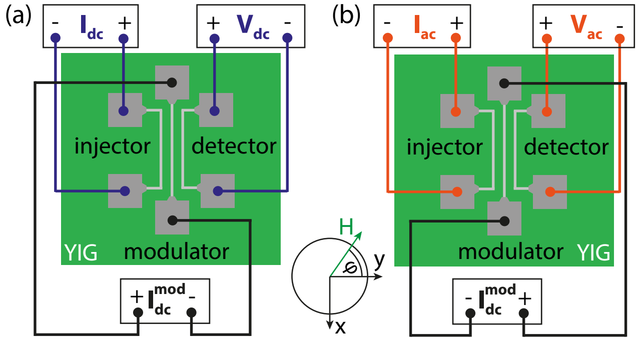


FIG. S1. Schematic depiction of the device (top view), detailed connection scheme for (a) the dc and (b) the ac technique, and the in-plane coordinate system.

The measurement setup of the first scheme, the dc-detection technique, is schematically sketched in Fig. S1(a). In our experiments, a dc charge current $I^{\mathrm{inj}} = 100$ µA is applied to the injector using a Keithley 2400 Sourcemeter and a Keithley 2182 Nanovoltmeter is used to detect the magnon transport signal. Moreover, we vary the dc charge current $I_{\mathrm{dc}}^{\mathrm{mod}}$ applied to the modulator strip with a Keithley 2400 Sourcemeter to manipulate the magnon transport via a SHE induced spin accumulation and Joule heating effects. In contrast, for

the ac-readout technique depicted in Fig. S1(b), we used a Keithley 6221 current source to feed a low frequency ($f = 7.737\,\mathrm{Hz}$) ac charge current $I_{\mathrm{ac}}^{\mathrm{inj}}(t)$ with a peak amplitude of 100 µA through the injector. The measured voltage signal at the detector is preamplified by a Standford Research System SR560 low-noise voltage amplifier before being passed to a Zurich Instruments HF2LI lock-in amplifier. Again, the dc current $I_{\mathrm{dc}}^{\mathrm{mod}}$ applied to the modulator is varied using a Keithley 2400 Sourcemeter. All measurements are conducted at $T = 280\,\mathrm{K}$.

## II. MEASUREMENT RESULTS OF THE SHE INJECTED MAGNONS FROM SAMPLE D300

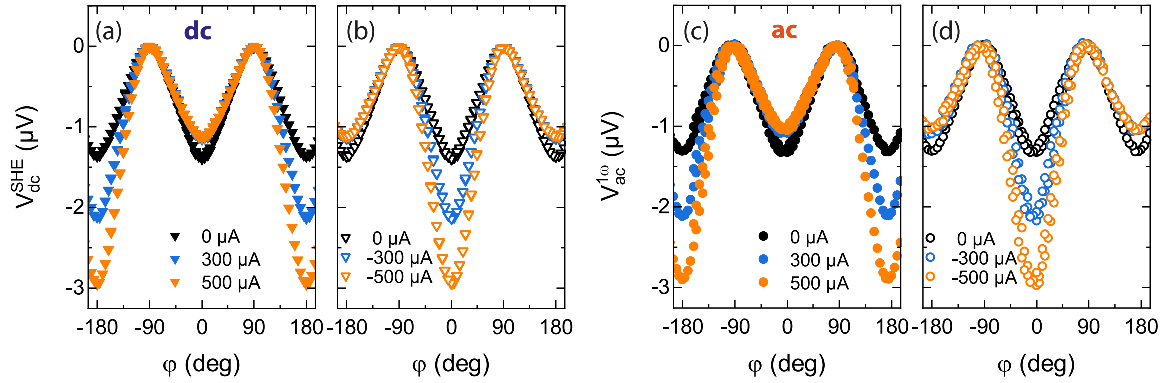


FIG. S2. (a), (b) Detector signals $V_{\mathrm{dc}}^{\mathrm{SHE}}$ and (c), (d) $V_{\mathrm{ac}}^{1\omega}$ plotted versus the rotation angle $\varphi$ of the in-plane magnetic field $\mathbf{H}$ measured with constant magnitude $\mu_0 H = 50\,\mathrm{mT}$ for various $I_{\mathrm{dc}}^{\mathrm{mod}}$. (a), (c) For $I_{\mathrm{dc}}^{\mathrm{mod}} > 0$ the magnon transport signal is significantly increased at $\varphi = \pm 180°$ and reduced at $\varphi = 0°$. (b), (d) For $I_{\mathrm{dc}}^{\mathrm{mod}} < 0$ we observe a 180° shifted behavior. The ranges and behavior of the SHE induced magnon transport signals $V_{\mathrm{dc}}^{\mathrm{SHE}}$ and $V_{\mathrm{ac}}^{1\omega}$ are in perfect agreement.

In this Section, we present our measurement results of sample D300 investigating the SHE injected magnons. To characterize the device, the detector voltage signals $V_{\mathrm{dc}}^{\mathrm{SHE}}$ and $V_{\mathrm{ac}}^{1\omega}$ are plotted as a function of the magnetic field orientation $\varphi$ measured with a magnetic field strength of $\mu_0 H = 50\,\mathrm{mT}$ for various $I_{\mathrm{dc}}^{\mathrm{mod}}$ in Fig. S2. The angle dependence of $V_{\mathrm{dc}}^{\mathrm{SHE}}$ and $V_{\mathrm{ac}}^{1\omega}$ perfectly agree with our results of sample D500 presented in the main text. While the magnon transport between injector and detector reveals the $\cos^2\varphi$ modulation for $I_{\mathrm{dc}}^{\mathrm{mod}} = 0$ (black data points) [S1, S2], we observe a significant enhancement at

$\varphi = \pm 180°$ for positive charge currents $I_{dc}^{mod} > 0$ at the modulator for $V_{dc}^{SHE}$ (Fig. S2(a)) as well as $V_{ac}^{1\omega}$(Fig. S2(c)). As already discussed in the main text, this enhancement can be attributed to a magnon accumulation underneath the modulator caused by the SHE induced magnon chemical potential and thermally generated magnons due to Joule heating, leading to an increase in magnon conductivity and therefore a larger magnon transport signal at the detector. Moreover, the decrease in the magnon transport signal at $\varphi = 0°$ for both techniques can be explained by a magnon depletion due to an annihilation of magnons via the SHE. However, the depletion is counterbalanced by thermally injected magnons caused by Joule heating of the modulator. For $I_{dc}^{mod} < 0$, $V_{dc}^{SHE}$ and $V_{ac}^{1\omega}$ plotted in Fig. S2(b) and (d), respectively, exhibit a 180° shifted behavior with an increased detector voltage signal for $\varphi = 0°$, while decreased at $\varphi = \pm 180°$. In both cases, the voltage amplitudes $V_{dc}^{SHE}$ and $V_{ac}^{1\omega}$ are in agreement for the dc and ac measurement scheme, as predicted by our model of the detector voltage signal.

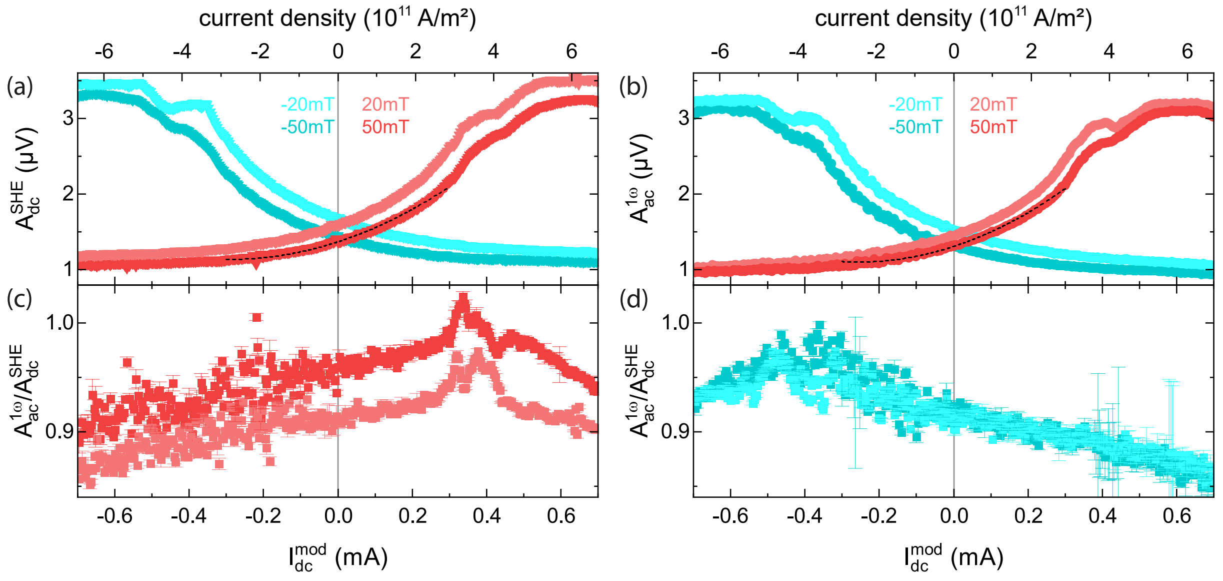


FIG. S3. Extracted amplitudes (a) $A_{dc}^{SHE}(\pm\mu_0 H)$ and (b) $A_{ac}^{1\omega}(\pm\mu_0 H)$ of the SHE injected magnon transport signal each plotted for different external magnetic fields versus the dc charge current $I_{dc}^{mod}$. The curves and the signal amplitudes show similar behaviors for (a) the dc and (b) the ac scheme. The black dashed line for $\mu_0 H = 50\,\mathrm{mT}$ is a fit indicating the $I_{dc}^{mod} + I_{dc}^{mod\,2}$ dependence in the low bias regime ($|I_{dc}^{mod}| \leq 0.3\,\mathrm{mA}$). (c), (d) Ratio $A_{ac}^{1\omega}/A_{dc}^{SHE}$ of the extracted amplitudes for the ac and dc configuration for (c) positive and (d) negative magnetic field magnitudes $\mu_0 H$.

Analogous to Figure 3 in the main text, we extract the amplitudes $A_{\rm dc}^{\rm SHE}(\pm\mu_0 H)$ and $A_{\rm ac}^{1\omega}(\pm\mu_0 H)$ of the angle-dependent measurements shown in Fig. S2 and plot them as a function of the applied modulator current $I_{\rm dc}^{\rm mod}$ for $|\mu_0 H| = 20\,{\rm mT}, 50\,{\rm mT}$ in Fig. S3. In accordance with our previous observations, we observe similar behaviors and detector voltage ranges for the dc (Fig. S3(a)) and ac (Fig. S3(a)) technique. In the low bias regime of sample D300 ($|I_{\rm dc}^{\rm mod}| \leq 0.3\,{\rm mA}$) we observe the predicted superposition of a linear (SHE) and quadratic (Joule heating) dependence. The fitted curve (black dashed line) for $\mu_0 H = 50\,{\rm mT}$ in Fig. S3(a) and (b) highlights the $I_{\rm dc}^{\rm mod} + {I_{\rm dc}^{\rm mod}}^2$ dependence in the low bias regime. We observe a clear deviation from this behavior for modulator currents $|I_{\rm dc}^{\rm mod}| > 0.3\,{\rm mA}$. For a quantitative comparison of the absolute amplitude values, we plot the ratio $A_{\rm ac}^{1\omega}/A_{\rm dc}^{\rm SHE}$ as a function of $I_{\rm dc}^{\rm mod}$ for positive and negative field amplitudes in Fig. S3(c) and (d), respectively. Focusing on $\mu_0 H = 50\,{\rm mT}$, we observe a slight increase of $A_{\rm ac}^{1\omega}/A_{\rm dc}^{\rm SHE}$ in the negative and low bias regime $I_{\rm dc}^{\rm mod} \leq 0.3\,{\rm mA}$. This behavior differs from the constant value observed for sample D500 over the whole modulator current range. However, the value is still close to 1, which is predicted by our model for the case that $R_j^{\text{inj-det}}\left(I_{\rm dc}^{\rm mod}\right) = 0$ for $j \geq 2$. Note, in contrast to sample D500, the measurements for D300 have been conducted in two different experimental setups for the dc and ac method, potentially causing differences in the detector resistances, which may explain the small deviation from the expected constant behavior. For modulator currents $I_{\rm dc}^{\rm mod} > 0.3\,{\rm mA}$, we observe a clear deviation from the behavior in the negative and low bias regime, indicating the contribution of higher order transport coefficients $R_j^{\text{inj-det}}\left(I_{\rm dc}^{\rm mod}\right) \neq 0$ (for $j \geq 2$), as discussed in the main text. While for $\mu_0 H = 20\,{\rm mT}$ the ratio shows a similar dependence, we extract a decrease of the ratio $A_{\rm ac}^{1\omega}/A_{\rm dc}^{\rm SHE}$ in the low and positive bias regime ($I_{\rm dc}^{\rm mod} \geq -0.3\,{\rm mA}$) for negative field polarity (Fig. S3(d)) and a threshold behavior for negative modulator currents $I_{\rm dc}^{\rm mod} < -0.3\,{\rm mA}$. The detector voltage signals of sample D300 nicely agree with our theoretical model, just as for sample D500, giving higher confidence comparing results obtained with different measurement techniques.

## III. ANGLE DEPENDENCE OF THE DETECTOR SIGNALS FROM SAMPLE D500 FOR NEGATIVE POLARITY

Having discussed the angle dependence of sample D500 for positive modulator charge currents ($I_{\rm dc}^{\rm mod} > 0$) for SHE and thermally injected magnons in the main text, we here

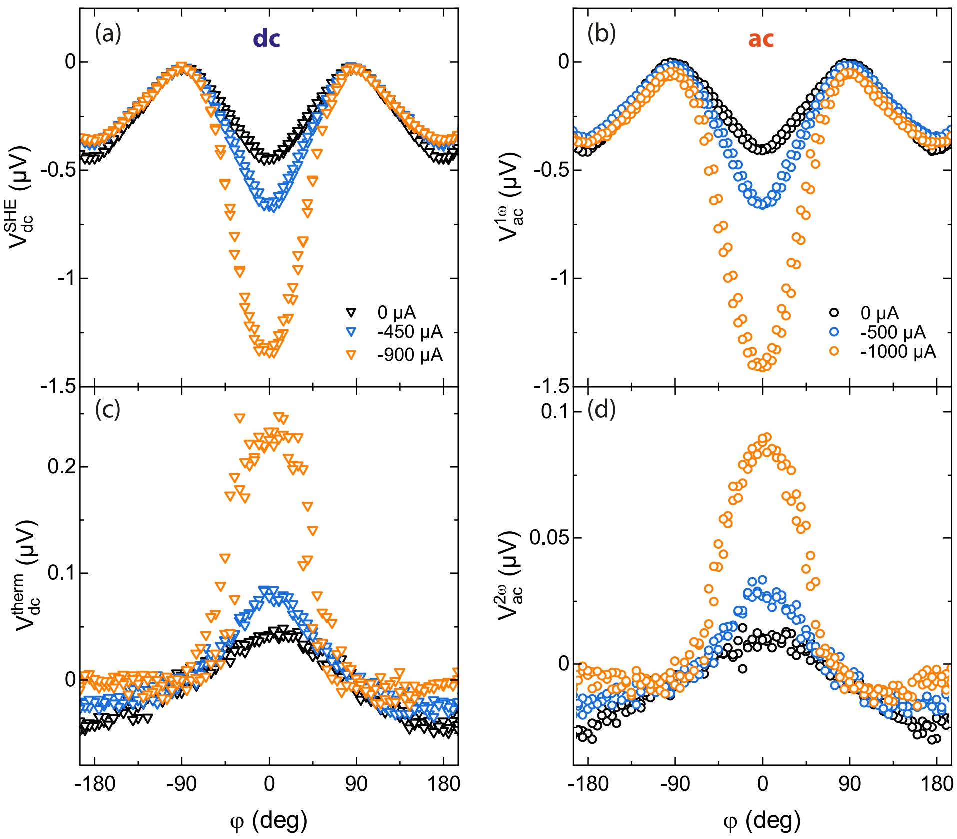


FIG. S4. Detector signals (a) $V_{\mathrm{dc}}^{\mathrm{SHE}}$, (b) $V_{\mathrm{ac}}^{1\omega}$, (c) $V_{\mathrm{dc}}^{\mathrm{therm}}$, (d) $V_{\mathrm{ac}}^{2\omega}$ plotted versus the rotation angle $\varphi$ of the in-plane magnetic field $\mathbf{H}$ with constant magnitude $\mu_0 H = 50\,\mathrm{mT}$ for various negative modulator currents $I_{\mathrm{dc}}^{\mathrm{mod}}$. For $I_{\mathrm{dc}}^{\mathrm{mod}} < 0$ the magnon transport signal is significantly increased at $\varphi = 0°$ and reduced at $\varphi = \pm 180°$. For the SHE induced magnon transport signals (a) $V_{\mathrm{dc}}^{\mathrm{SHE}}$ and (b) $V_{\mathrm{ac}}^{1\omega}$, the behavior and the ranges of the voltage signals are perfectly in agreement. While the angle dependence of the thermal signals (c) $V_{\mathrm{dc}}^{\mathrm{therm}}$ and (d) $V_{\mathrm{ac}}^{2\omega}$ is in good agreement, their absolute amplitude values strongly differ.

concentrate on the negative current polarity ($I_{\mathrm{dc}}^{\mathrm{mod}} < 0$). In Fig. S4(a) and (b), we plot $V_{\mathrm{dc}}^{\mathrm{SHE}}$ and $V_{\mathrm{ac}}^{1\omega}$, respectively, as a function of the in-plane angle $\varphi$ for various negative $I_{\mathrm{dc}}^{\mathrm{mod}}$. For $I_{\mathrm{dc}}^{\mathrm{mod}} < 0$, we observe a 180° shifted behavior compared to Figure 2 in the main text for $I_{\mathrm{dc}}^{\mathrm{mod}} > 0$, i.e. the magnon transport signal for $V_{\mathrm{dc}}^{\mathrm{SHE}}$ and $V_{\mathrm{ac}}^{1\omega}$ is significantly increased at $\varphi = 0°$, while it is decreased at $\varphi = \pm 180°$, as already reported in Ref. S3. In this configuration, the increase at $\varphi = 0°$ originates from a magnon accumulation underneath the modulator caused by the SHE induced magnon chemical potential and thermally generated magnons due to Joule heating. The decrease at $\varphi = \pm 180°$ is caused by a magnon depletion

via the annihilation of magnons via the SHE, which is however counterbalanced by thermally injected magnons at the modulator. As for positive modulator charge currents, not just the behavior of $V_{\mathrm{dc}}^{\mathrm{SHE}}$ and $V_{\mathrm{ac}}^{1\omega}$ are in good agreement for $I_{\mathrm{dc}}^{\mathrm{mod}} < 0$, but also the ranges of the voltage signals.

For the same reasons, the voltage signals of the thermally injected magnons $V_{\mathrm{dc}}^{\mathrm{therm}}$ (Fig. S4(c)) and $V_{\mathrm{ac}}^{2\omega}$ (Fig. S4(d)) are increased at $\varphi = 0°$ and decreased at $\varphi = \pm 180°$. In agreement with our previous observations and our model, we observe that $V_{\mathrm{dc}}^{\mathrm{therm}}$ and $V_{\mathrm{ac}}^{2\omega}$ strongly differ in their absolute amplitude values (for quantitative comparison see section IV).

## IV. SHE AND THERMALLY INJECTED MAGNONS FOR VARYING FIELDS

In the main text, we investigate $A_{\mathrm{dc}}^{\mathrm{SHE}}$, $A_{\mathrm{ac}}^{1\omega}$, $A_{\mathrm{dc}}^{\mathrm{therm}}$, $A_{\mathrm{ac}}^{2\omega}$ for $\mu_0 H = 60\,\mathrm{mT}$ to quantitatively compare the dc and ac scheme. In this section, we investigate the field dependence of these amplitude voltage signals. We first focus on $A_{\mathrm{dc}}^{\mathrm{SHE}}(\pm\mu_0 H)$ and $A_{\mathrm{ac}}^{1\omega}(\pm\mu_0 H)$ plotted as a function of $I_{\mathrm{dc}}^{\mathrm{mod}}$ in Fig. S5(a) and (b) for various magnetic field amplitudes $\mu_0 H$. For all applied fields $\mu_0 H$, we observe a similar behavior compared to $\mu_0 H = 60\,\mathrm{mT}$, discussed in the main text. In the low bias regime ($|I_{\mathrm{dc}}^{\mathrm{mod}}| \leq 0.55\,\mathrm{mT}$), the detector signal amplitudes can be modeled by a superposition of a linear (SHE) and quadratic (Joule heating) dependence, while for $|I_{\mathrm{dc}}^{\mathrm{mod}}| > 0.55\,\mathrm{mT}$ we observe a clear deviation from this behavior. The calculated ratios $A_{\mathrm{ac}}^{1\omega}/A_{\mathrm{dc}}^{\mathrm{SHE}}$ are shown in Fig. S5(c), (e) for positive and in (d), (f) for negative magnetic field magnitudes. For positive magnetic field magnitudes we observe a similar modulator current dependence of $A_{\mathrm{ac}}^{1\omega}/A_{\mathrm{dc}}^{\mathrm{SHE}}$ as for $\mu_0 H = 60\,\mathrm{mT}$. In the low and negative bias regime ($I_{\mathrm{dc}}^{\mathrm{mod}} \leq 0.55\,\mathrm{mA}$) the ratios are nearly constant. Although the ratios in this regime exhibit slightly varying values for different magnetic fields $\mu_0 H$, all are close to 1, as predicted by our theoretical model. We extract a clear deviation from 1 for $I_{\mathrm{dc}}^{\mathrm{mod}} > 0.55\,\mathrm{mT}$, when higher orders of $I^{\mathrm{inj}}$ contribute. For negative magnetic field magnitudes a similar dependence of $A_{\mathrm{ac}}^{1\omega}/A_{\mathrm{dc}}^{\mathrm{SHE}}$ can be extracted, however with a polarity change in $I_{\mathrm{dc}}^{\mathrm{mod}}$ and thus a threshold for negative modulator currents $I_{\mathrm{dc}}^{\mathrm{mod}}$. Our results for various magnetic fields are in agreement with our previous observation and our theoretical model [S3]. The model predicts a ratio $A_{\mathrm{ac}}^{1\omega}/A_{\mathrm{dc}}^{\mathrm{SHE}}$ of 1 in the case that $R_j^{\text{inj-det}}\left(I_{\mathrm{dc}}^{\mathrm{mod}}\right) = 0$ for $j \geq 2$, while the deviation for higher

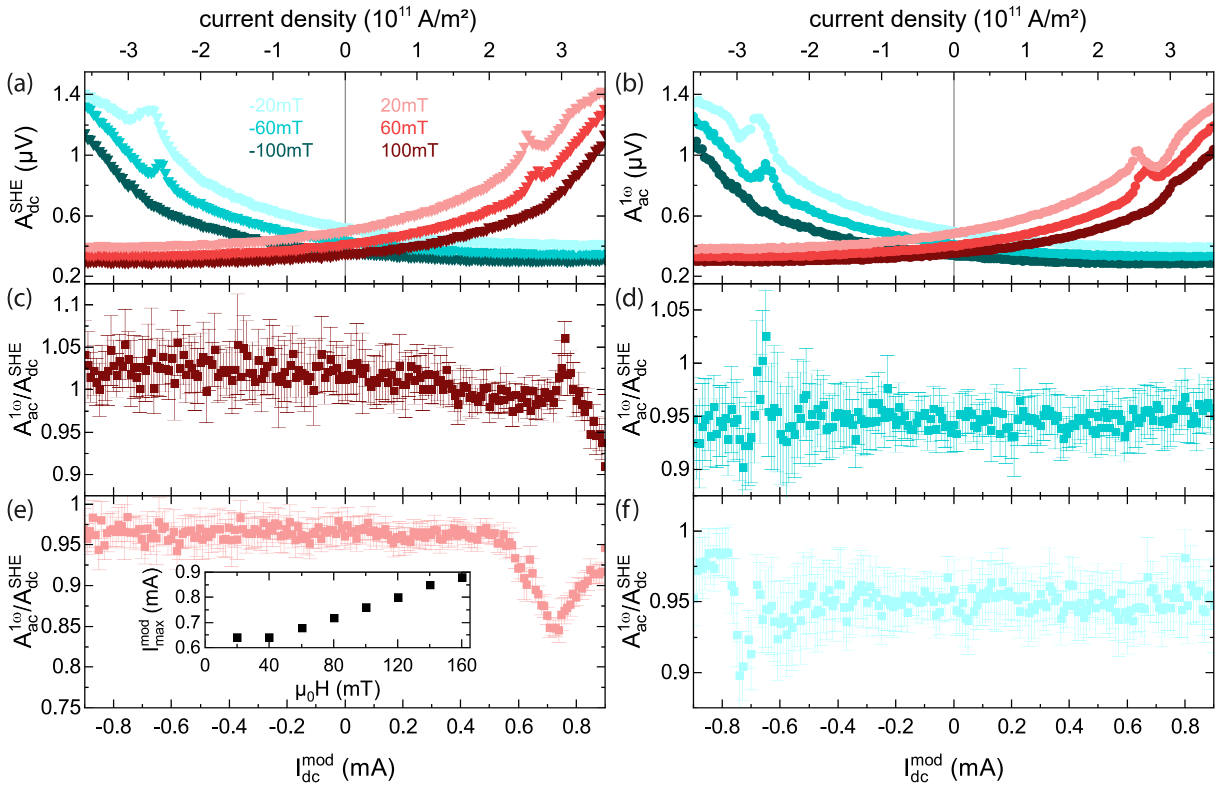


FIG. S5. Extracted amplitudes (a) $A_{\mathrm{dc}}^{\mathrm{SHE}}(\pm\mu_0 H)$ and (b) $A_{\mathrm{ac}}^{1\omega}(\pm\mu_0 H)$ of the SHE injected magnon transport signal each plotted for various external magnetic fields $\mu_0 H$ versus the dc charge current $I_{\mathrm{dc}}^{\mathrm{mod}}$. The curves and signal amplitudes show similar behaviors for (a) the dc and (b) the ac scheme. (c), (d), (e), (f) Ratio $A_{\mathrm{ac}}^{1\omega}/A_{\mathrm{dc}}^{\mathrm{SHE}}$ of the extracted amplitudes for the ac and dc configuration for (c), (e) positive and (d), (f) negative magnetic field amplitudes $\mu_0 H$. (c), (e) For $I_{\mathrm{dc}}^{\mathrm{mod}} \leq 0.55\,\mathrm{mA}$ the ratio exhibits a nearly constant behavior close to the value 1. We observe a clear deviation from 1 for higher modulator charge current values. (d), (f) For $\mu_0 H < 0$ we extract a similar dependence with a threshold for negative modulator charge currents ($I_{\mathrm{dc}}^{\mathrm{mod}} < -0.55\,\mathrm{mA}$). (e) The inset shows $I_{\mathrm{max}}^{\mathrm{mod}}$ the maximum of the ratio $A_{\mathrm{ac}}^{1\omega}/A_{\mathrm{dc}}^{\mathrm{SHE}}$ for $I_{\mathrm{dc}}^{\mathrm{mod}} > 0.55\,\mathrm{mA}$ as a function of the applied magnetic field $\mu_0 H$.

modulator currents ($I_{\mathrm{dc}}^{\mathrm{mod}} > 0.55\,\mathrm{mA}$) indicates a deviation from the linear dependence and contributions of higher order terms in $I^{\mathrm{inj}}$.

For a more quantitative analysis of the field dependence, we extract for the nonlinear regime ($I_{\mathrm{dc}}^{\mathrm{mod}} > 0.55\,\mathrm{mA}$) the modulator current $I_{\mathrm{max}}^{\mathrm{mod}}$ taken at the current level where the ratio level reaches its maximum. The determined modulator currents $I_{\mathrm{max}}^{\mathrm{mod}}$ are plotted as a function of the applied magnetic field in the inset of Fig. S5(e). We observe a constant

behavior around a modulator current of 0.64 mA for $\mu_0 H < 40$ mT, while for larger magnetic field strengths $\mu_0 H > 40$ mT $I_{\rm max}^{\rm mod}$ increases with the applied magnetic field. Similar results have been observed in our previous work for the critical threshold currents [S3].

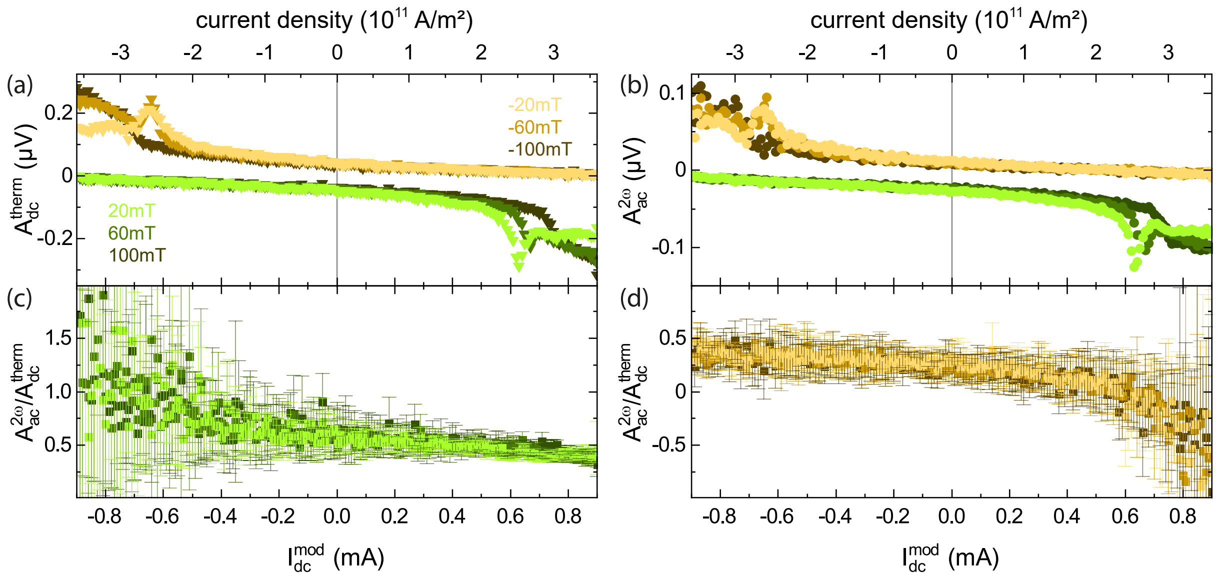


FIG. S6. Extracted amplitudes (a) $A_{\rm dc}^{\rm therm}(\pm\mu_0 H)$ and (b) $A_{\rm ac}^{2\omega}(\pm\mu_0 H)$ of the thermally generated magnon transport signal each plotted for different external magnetic fields versus the dc charge current $I_{\rm dc}^{\rm mod}$. (c), (d) Ratio $A_{\rm ac}^{2\omega}/A_{\rm dc}^{\rm therm}$ of the extracted amplitudes for the ac and dc configuration for (c) positive and (d) negative magnetic field amplitudes $\mu_0 H$. In both cases the ratio exhibits a nearly constant behavior over the whole modulator current range at a value close to 0.5 within the experimental error.

We now discuss the voltage signals $A_{\rm dc}^{\rm therm}(\pm\mu_0 H)$ and $A_{\rm ac}^{2\omega}(\pm\mu_0 H)$ of the thermally induced magnons, plotted as a function of $I_{\rm dc}^{\rm mod}$ for the same multiple magnetic fields $\mu_0 H$ as in the case of the SHE injected magnons $A_{\rm dc}^{\rm SHE}$ and $A_{\rm ac}^{1\omega}$. The qualitative dependence on $I_{\rm dc}^{\rm mod}$ is identical for $A_{\rm dc}^{\rm therm}$, $A_{\rm ac}^{2\omega}$ for all investigated magnetic fields and current ranges. In all cases, we find a significant kink above a critical current value, as reported in previous works [S3]. For a more quantitative comparison the ratio of the extracted signal amplitudes $A_{\rm ac}^{2\omega}/A_{\rm dc}^{\rm therm}$ is plotted in Fig. S6(c) and (d) for positive and negative magnetic field polarity, respectively, as a function of $I_{\rm dc}^{\rm mod}$. Independent of $\mu_0 H$, $A_{\rm ac}^{2\omega}/A_{\rm dc}^{\rm therm}$ exhibits a nearly constant behavior over the whole modulator current range. As for $\mu_0 H = 60$ mT, the ratios $A_{\rm ac}^{2\omega}/A_{\rm dc}^{\rm therm}$ for various magnetic fields are close to 0.5 within the experimental error, nicely in accordance

with our simple model of the detector voltage signal. While we observe a magnetic field dependence for $A_{\mathrm{ac}}^{1\omega}/A_{\mathrm{dc}}^{\mathrm{SHE}}$, the ratio $A_{\mathrm{ac}}^{2\omega}/A_{\mathrm{dc}}^{\mathrm{therm}}$ shows no dependence on the magnetic field magnitude.

## V. THIRD HARMONIC VOLTAGE SIGNAL

As stated in the main text, $V_{\mathrm{dc}}^{\mathrm{SHE}}$ and $V_{\mathrm{ac}}^{1\omega}$ should be identical if $R_j^{\text{inj-det}} = 0$ for $j \geq 2$. However, if we assume an additional third order contribution in $I^{\mathrm{inj}}$, i.e. the finite transport coefficient $R_3^{\text{inj-det}} \neq 0$, one would expect within our model to observe a signal in the third harmonic. When we use equation (2) and (4) in the main text and only consider contribution up to the third order, the difference of the two voltages can be calculated to $V_{\mathrm{dc}}^{\mathrm{SHE}} - V_{\mathrm{ac}}^{1\omega} = 1/4 R_3^{\text{inj-det}} {I^{\mathrm{inj}}}^3$. From the difference of $A_{\mathrm{dc}}^{\mathrm{SHE}}$ and $A_{\mathrm{ac}}^{1\omega}$ we can estimate a third harmonic signal of the order of several 10 nV, which is unfortunately lower than the noise floor in our lock-in measurements. Thus, we could not detect any significant third harmonic signal, but improvements in signal-to-noise ratio may allow the detection of this higher order contribution.

---


[S1] L. J. Cornelissen, J. Liu, R. A. Duine, J. B. Youssef, and B. J. van Wees, Nature Physics **11**, 1022 (2015).

[S2] S. T. B. Goennenwein, R. Schlitz, M. Pernpeintner, K. Ganzhorn, M. Althammer, R. Gross, and H. Huebl, Applied Physics Letters **107**, 172405 (2015).

[S3] T. Wimmer, M. Althammer, L. Liensberger, N. Vlietstra, S. Geprägs, M. Weiler, R. Gross, and H. Huebl, Phys. Rev. Lett. **123**, 257201 (2019).
